# Supplementary material for: DexGraspNet 2.0: Learning Generative Dexterous Grasping in Large-scale Synthetic Cluttered Scenes
Source: arXiv:2410.23004 source file (2024-10-30)
Supplement: Supplementary file 1 [file supp99_Video.tex]

\section{[describe our supp video]}
